# Supplementary material for: Exploring Modality Guidance to Enhance VFM-based Feature Fusion for UDA in 3D Semantic Segmentation
Source: arXiv:2504.14231 source file (2025-04-19)
Supplement: Supplementary file 1 [file X_suppl.tex]

%\clearpage
%\setcounter{page}{1}
%\maketitlesupplementary

% \section{Introduction}
% \label{sec:supplementary}
In the following, we provide additional complimentary resources for our work. First, we provide an extended baseline fusion comparison (Section ~\ref{sec:extended_baseline_comparison}). 
Then for additional insights, we provide ablation of the prediction aggregation (Section~\ref{sec:study_prediction_aggregation}). 
% \wei{introduction to complete ... add section number}
In addition, we extend our ablation of modality guidance within the source domain (Section~\ref{sec:modality_guidance_source}). 
Finally, we provide additional details of the datasets (Section~\ref{sec:dataset_details}). 

To ensure reproducibility, we provide our complete codebase as \texttt{code.zip} in addition to the supplementary document. 
The codebase also contains a detailed \texttt{readme.md} that contains instructions on reproducing the main results reported in our paper.

% \paragraph{Extended Baseline Comparison.}
\section{Extended Baseline Comparison}\label{sec:extended_baseline_comparison}
We conduct a comparison to our baseline fusion evaluation and report results on three Domain Adaptation (DA) datasets in Table~\ref{tab:xmuda_supplementory_comparison} (as an extension to Table~3 in the main manuscript). 
For completeness, here we additionally include the variant~\textit{xMUDA-VFM} which is the vanilla xMUDA (non-fusion)~\cite{jaritz2022cross} with the frozen Visual Foundation Model (VFM) RADIO-AM \cite{ranzinger2024radio} as the 2D backbone. 
This is done to ensure a direct comparison with our method. 
% Due to the absence of the trainable 2D backbone for xMUDA-VFM, we apply the cross-modal alignment on the VFM main head as outlined in \cite{jaritz2022cross} as a baseline alternative.

% The results summarize deficiencies of the existing xMUDA variants that arise due to incompatibilities with a frozen backbone which our method overcomes. 
The results highlight the limitations of existing xMUDA variants, which stem from their incompatibility with a frozen VFM backbone - an issue effectively addressed by our method. 
Notably, our approach surpasses \textit{xMUDA-VFM-Fuse} across all DA scenarios, with a notable improvement of 6.2\% for the \emph{Day $\to$ Night} adaptation.
% Our method outperforms \textit{xMUDA-VFM-Fuse} in all the four DA scenarios, especially on the \emph{Day $\to$ Night} evaluation where our method demonstrates a significant improvement of 6.2\%. 
% While we outperform \textit{xMUDA-VFM-Fuse} only moderately on the tasks where the VFM is the stronger modality, we adapt significantly better than the the xMUDA fusion in the \emph{Day $\to$ Night} scenario. 
On the other hand, the \textit{xMUDA-VFM} shows only marginally reduced performance compared to us on the 3D dataset, but is significantly hampered in the VFM dominant tasks, due to the cross-modal alignment of the 2D main head which degrades the performance. This supports our design choice to refrain from applying a cross-modal alignment to our VFM main classifier. Further, the xMUDA-VFM is also not able to leverage a refined fusion representation. 
\begin{table}[t!]
\footnotesize
  \centering
\begin{tabular}{l|c|c|c}
\toprule
    2D3D  & USA $\to$ Sing. & Day $\to$ Night &  A2D2 $\to$ SK \\ 
     \midrule \midrule%\cline{2-5} 

xMUDA \cite{jaritz2022cross}  & 69.2 & 67.4 &  44.0 \\
xMUDA-Fuse \cite{jaritz2022cross}  &  69.3 & -  & 42.6  \\
xMUDA-VFM & 63.2 & 69.1  & 53.7  \\
xMUDA-VFM-F. & 73.4 & 64.1   & 61.4 \\
\midrule
Ours   & 74.6 & 70.3 &  63.1 \\ 
\bottomrule
\bottomrule
\end{tabular}
\caption{Extended comparison of xMUDA and xMUDA-Fuse variants with and without VFM backbone. For xMUDA-VFM and xMUDA-VFM-Fuse the trainable 2D backbone is replaced with a frozen VFM. For xMUDA-VFM the cross modal predictive alignment is applied on the 2D main head.  }

\label{tab:xmuda_supplementory_comparison}
\end{table}
\begin{table*}[t!]
\centering
\begin{tabular}{c|c}
\toprule
\textbf{Task}                 &  \textbf{Merged Classes}                           \\ \midrule
nuScenes derivations                  & Vehicle, Drivable Surface, Sidewalk, Terrain, Manmade, Vegetation    \\     

A2D2 $\to$ SK          & Car, Truck, Bike, Person, Road, Parking, Sidewalk, Building, Nature, Other-Objects                      \\ 
VK $\to$ SK    & Car, Truck, Road, Vegetation/Terrain, Building, Object                                                   \\ 
\bottomrule

\end{tabular}
\caption{List of classes for each task (excluding ignore and unlabeled classes). Both \emph{Day $\to$ Night} and \emph{USA $\to$ Singapore} use the same class mapping. }
\label{tab:merged_classes_tasks}
\end{table*}

\begin{figure}[ht]
    \centering
    \includegraphics[width=\columnwidth]{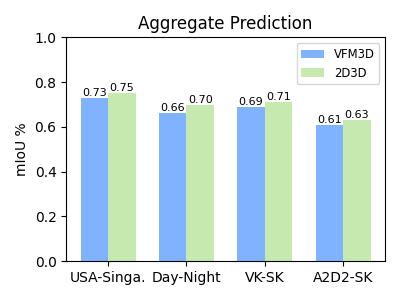}
    \caption{Comparison to an alternative prediction aggregation for the final prediction. 
      We compare the softmax average of our VFM classifier and the fusion main classifier when added to the 3D prediction.}
    \label{fig:aggregate_performance}
\end{figure}
\begin{table}
%\small
  \centering
\setlength{\tabcolsep}{3pt}
\begin{tabular}{l|ccc}
\toprule
   \multirow{2}{*}{Method}  & \multicolumn{3}{c}{VK $\to$ SK}\\ 
 &  2D & 3D & 2D3D  \\  \midrule\midrule%\cline{2-5} 
Source \cite{jaritz2022cross} & 26.8 & 42.0 & 42.2 \\
Source w\textbackslash o MG &  64.0 &  32.5 &  59.4\\
Source + MG &  64.9 &  29.0 &  59.9 \\ 
\midrule
Ours & 70.1 & 64.5 & 70.7\\ 

\bottomrule
\bottomrule
\end{tabular}%}
\caption{Source comparison. The regularizing effect of the modality guidance (MG) is setting in full when the target data is applied. }
\label{tab:source_comparision}
\end{table}
\begin{table}[ht]
\centering
\begin{tabular}{l|c|ccc}
\toprule
\multirow{2}{*}{Task} & \multicolumn{1}{c}{Source} & \multicolumn{3}{c}{Target} \\
& Train & Train & Val & Test \\
\midrule
\midrule
USA $\to$ Sing. & 15,695 & 9,665 & 2,770 & 2,929 \\
Day $\to$ Night & 24,745 & 2,779 & 606 & 602 \\
VK $\to$ SK & 2,126 & 18,029 & 1,101 & 4,071 \\
A2D2 $\to$ SK & 27,695 & 18,029 & 1,101 & 4,071 \\
\bottomrule
\bottomrule
\end{tabular}
\caption{ Number of images per dataset split per task. }
\label{tab:dataset_task_splits}
\end{table}

\section{Study on Prediction Aggregation}\label{sec:study_prediction_aggregation}
In Figure~\ref{fig:aggregate_performance} we show additional results from our main experiment to compare our choice of the final prediction from the individual classifier heads. We compare the softmax average of the VFM and 3D as a potential alternative to the final prediction, the softmax average of the fusion and 3D predictions. 

The results show that the utilization of our refined fusion head leads to improved performance over combining the 3D predictions with the VFM classifier in all tasks, most pronounced in the \emph{Day$\to$Night} task. Overall the performance of VFM3D is similar to the performance of XMUDA-VFM-Fuse, which we outperform on average by 3\% over the three tasks.

\section{Modality Guidance on Source}\label{sec:modality_guidance_source}
In Table~\ref{tab:source_comparision} we provide the results of our method on source only, including the cross modal losses, and ablate the impact of the modality guiding loss. While the results are improved with the modality guidance, overall the modality guidance's regularizing effect is stronger on a domain shift on target data. However, on source, there is little signal to focus the representation based on one modality, since the guidance loss can likely be minimized well relying on in domain features from both modalities.

\section{Dataset Details}~\label{sec:dataset_details}
In Table~\ref{tab:dataset_task_splits} we report the number of images per dataset split. It is noteworthy that the VirtualKITTI~\cite{gaidon2016virtualkitti} (source) training split contains comparatively few images. Also, the nuScenes~\cite{caesar2020nuscenes} Night (target) is comparatively small, with the test and validation split containing only 602 images.
In Table~\ref{tab:merged_classes_tasks} we list the merged classes for each task.

%16 nuscenes
%a2d2 38
%sk 33

%Dataset classes
%Dataset Observations
%Datset class merges
%Lidar Beams

%\paragraph{Additional VFMS}
%\input{fig_tex/compare_model_performance_supplementory}
