# Supplementary material for: Exploring Modality Guidance to Enhance VFM-based Feature Fusion for UDA in 3D Semantic Segmentation
Source: arXiv:2504.14231 source file (2025-04-19)
Supplement: Supplementary file 2 [file aggregate_performance_supplementory.tex]

\begin{figure}[ht]
    \centering
    \includegraphics[width=\columnwidth]{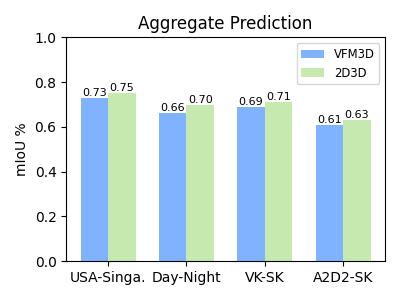}
    \caption{Comparison to an alternative prediction aggregation for the final prediction. 
      We compare the softmax average of our VFM classifier and the fusion main classifier when added to the 3D prediction.}
    \label{fig:aggregate_performance}
\end{figure}
