# Supplementary material for: Exploring Modality Guidance to Enhance VFM-based Feature Fusion for UDA in 3D Semantic Segmentation
Source: arXiv:2504.14231 source file (2025-04-19)
Supplement: Supplementary file 4 [file classes_supplementory.tex]

\begin{table*}[t!]
\centering
\begin{tabular}{c|c}
\toprule
\textbf{Task}                 &  \textbf{Merged Classes}                           \\ \midrule
nuScenes derivations                  & Vehicle, Drivable Surface, Sidewalk, Terrain, Manmade, Vegetation    \\     

A2D2 $\to$ SK          & Car, Truck, Bike, Person, Road, Parking, Sidewalk, Building, Nature, Other-Objects                      \\ 
VK $\to$ SK    & Car, Truck, Road, Vegetation/Terrain, Building, Object                                                   \\ 
\bottomrule

\end{tabular}
\caption{List of classes for each task (excluding ignore and unlabeled classes). Both \emph{Day $\to$ Night} and \emph{USA $\to$ Singapore} use the same class mapping. }
\label{tab:merged_classes_tasks}
\end{table*}
