# Supplementary material for: Exploring Modality Guidance to Enhance VFM-based Feature Fusion for UDA in 3D Semantic Segmentation
Source: arXiv:2504.14231 source file (2025-04-19)
Supplement: Supplementary file 5 [file compare_to_xmuda_supplementory.tex]

\begin{table}[t!]
\footnotesize
  \centering
\begin{tabular}{l|c|c|c}
\toprule
    2D3D  & USA $\to$ Sing. & Day $\to$ Night &  A2D2 $\to$ SK \\ 
     \midrule \midrule%\cline{2-5} 

xMUDA \cite{jaritz2022cross}  & 69.2 & 67.4 &  44.0 \\
xMUDA-Fuse \cite{jaritz2022cross}  &  69.3 & -  & 42.6  \\
xMUDA-VFM & 63.2 & 69.1  & 53.7  \\
xMUDA-VFM-F. & 73.4 & 64.1   & 61.4 \\
\midrule
Ours   & 74.6 & 70.3 &  63.1 \\ 
\bottomrule
\bottomrule
\end{tabular}
\caption{Extended comparison of xMUDA and xMUDA-Fuse variants with and without VFM backbone. For xMUDA-VFM and xMUDA-VFM-Fuse the trainable 2D backbone is replaced with a frozen VFM. For xMUDA-VFM the cross modal predictive alignment is applied on the 2D main head.  }

\label{tab:xmuda_supplementory_comparison}
\end{table}
