# Supplementary material for: Exploring Modality Guidance to Enhance VFM-based Feature Fusion for UDA in 3D Semantic Segmentation
Source: arXiv:2504.14231 source file (2025-04-19)
Supplement: Supplementary file 6 [file head_comparison_supplementory.tex]

\begin{table*}
\centering
\small
{\begin{tabular}{l|cc|cc|cc|cc}
\toprule 
        & \multicolumn{2}{c}{USA $\to$ Singapore}
        & \multicolumn{2}{c}{Day $\to$ Night} 
        & \multicolumn{2}{c}{VK $\to$ SK} 
        & \multicolumn{2}{c}{A2D2 $\to$ SK}  \\ 
Method & VFM3D & 2D3D & VFM3D & 2D3D  & VFM3D & 2D3D & VFM3D & 2D3D   \\  \midrule \midrule%\cline{2-5} 
ours & 73.3 & 75.4 & 65.8 & 70.3 & 69.2& 70.7 & 61.3 & 63.1 \\
\end{tabular}}
\caption{Comparison of our heads} 
\label{tab:head_comparision}
\end{table*}
