# Supplementary material for: Exploring Modality Guidance to Enhance VFM-based Feature Fusion for UDA in 3D Semantic Segmentation
Source: arXiv:2504.14231 source file (2025-04-19)
Supplement: Supplementary file 7 [file source_ablation_supplementory.tex]

\begin{table}
%\small
  \centering
\setlength{\tabcolsep}{3pt}
\begin{tabular}{l|ccc}
\toprule
   \multirow{2}{*}{Method}  & \multicolumn{3}{c}{VK $\to$ SK}\\ 
 &  2D & 3D & 2D3D  \\  \midrule\midrule%\cline{2-5} 
Source \cite{jaritz2022cross} & 26.8 & 42.0 & 42.2 \\
Source w\textbackslash o MG &  64.0 &  32.5 &  59.4\\
Source + MG &  64.9 &  29.0 &  59.9 \\ 
\midrule
Ours & 70.1 & 64.5 & 70.7\\ 

\bottomrule
\bottomrule
\end{tabular}%}
\caption{Source comparison. The regularizing effect of the modality guidance (MG) is setting in full when the target data is applied. }
\label{tab:source_comparision}
\end{table}
