# Supplementary material for: Exploring Modality Guidance to Enhance VFM-based Feature Fusion for UDA in 3D Semantic Segmentation
Source: arXiv:2504.14231 source file (2025-04-19)
Supplement: Supplementary file 8 [file tasks_splits_supplementroy_2.tex]

\begin{table}[ht]
\centering
\begin{tabular}{l|c|ccc}
\toprule
\multirow{2}{*}{Task} & \multicolumn{1}{c}{Source} & \multicolumn{3}{c}{Target} \\
& Train & Train & Val & Test \\
\midrule
\midrule
USA $\to$ Sing. & 15,695 & 9,665 & 2,770 & 2,929 \\
Day $\to$ Night & 24,745 & 2,779 & 606 & 602 \\
VK $\to$ SK & 2,126 & 18,029 & 1,101 & 4,071 \\
A2D2 $\to$ SK & 27,695 & 18,029 & 1,101 & 4,071 \\
\bottomrule
\bottomrule
\end{tabular}
\caption{ Number of images per dataset split per task. }
\label{tab:dataset_task_splits}
\end{table}
